# Supplementary material for: Model-Free Linear Quadratic Control via Reduction to Expert Prediction
Source: arXiv:1804.06021 source file (2018-10-05)
Supplement: Supplementary file 1 [file appendix_qfun.tex]

\section{$Q$ function for linear quadratic systems}
\label{sec:q_fun}

\begin{lemma}
\label{lem:quadratic}
Let $\pi(x) = - K x$ be a linear policy such that $\norm{A-BK} < 1$. 
 The state-action value function of policy $\pi$ has the quadratic form
\[
Q_\pi(x,a) = 
\begin{pmatrix}
          x^\top\, a^\top
\end{pmatrix} 
G_\pi 
\begin{pmatrix}
           x \\
           a
\end{pmatrix}\,,
\] 
where $G_\pi$ is the unique symmetric solution of the equation 
\[
G_\pi = 
      S^\top G_\pi S
      +
      \begin{pmatrix}
        M & 0 \\
        0 & N 
       \end{pmatrix}\,, \quad
S = 
      \begin{pmatrix}
                 I \\
                 -K
      \end{pmatrix}
      \begin{pmatrix}
                A\,\,\, B
      \end{pmatrix}\,. 
\]
\end{lemma}
\begin{proof}
We prove the lemma by showing that the given quadratic form is the unique solution of the Bellman equation. Let 
\[
z = 
\begin{pmatrix}
           x \\
           a
\end{pmatrix}\,,\qquad 
z' = 
\begin{pmatrix}
x'\\
a'
\end{pmatrix}
=
\begin{pmatrix}
      A x + B a + w \\
      -K(A x + B a + w)
\end{pmatrix} \,,
\]  
be the current state-action and a random next state-action under policy $\pi$. We guess a quadratic form $z^\top G_\pi z + L^\top z$ for the value function and we write
\[
\lambda_\pi + 
\begin{pmatrix}
          x^\top\, a^\top
\end{pmatrix} 
G_\pi 
\begin{pmatrix}
           x \\
           a
\end{pmatrix}
+ 
L^\top 
\begin{pmatrix}
           x \\
           a
\end{pmatrix}
=
\begin{pmatrix}
          x^\top\, a^\top
\end{pmatrix} 
\begin{pmatrix}
  M & 0 \\
  0 & N 
 \end{pmatrix} 
\begin{pmatrix}
           x \\
           a
\end{pmatrix}
+ \E\left\{
\begin{pmatrix}
          x'^\top\, a'^\top
\end{pmatrix} 
G_\pi 
\begin{pmatrix}
           x' \\
           a'
\end{pmatrix}
+ 
L^\top 
\begin{pmatrix}
           x' \\
           a'
\end{pmatrix}
\right\} 
\;.
\]
By matching terms, we find that the above equation has a solution iff
\begin{align}
\lambda_\pi 
& = {\rm trace} \bigg(
            \begin{pmatrix}
                       I \\
                       -K
            \end{pmatrix}^\top\,
            G_\pi \,
            \begin{pmatrix}
                       I \\
                       -K
            \end{pmatrix} W\bigg)\,, 
            \nonumber \\
G_\pi &= 
            S^\top G_\pi S
            +
            \begin{pmatrix}
              M & 0 \\
              0 & N 
             \end{pmatrix}\,,
            \label{eq:G}  
             \\
L & =
              L S\,.
\label{eq:L}
\end{align}
We have that
\[
\norm{
\begin{pmatrix}
          A\,\,\, B
\end{pmatrix}
\begin{pmatrix}
           I \\
           -K
\end{pmatrix}
}
=
\norm{A - B K} < 1 \;.
\]
By the associativity of matrix products,
this implies that if we form iterations from equations \eqref{eq:G} and \eqref{eq:L}
where the right-hand side is reassigned to the left-hand side,
then this iteration converges. By continuity, it follows that the limit will satisfy the respective equations.
It also follows that these equations have unique solutions, and in particular $L=0$. Thus, the quadratic form as stated is the solution of the Bellman equation. 
\end{proof}

\iffalse
\section{Greedy policy for the average cost}
\label{sec:greedy_avg}

To find the greedy policy 
\begin{align*}
K_* &= \arg \max_{K} tr( 
\begin{bmatrix} I & -K^\top \end{bmatrix} 
\begin{bmatrix} G_{11} & G_{12} \\ G_{21} & G_{22} \end{bmatrix}
\begin{bmatrix} I \\ -K \end{bmatrix}
W)\\
&= \arg \max_{K} tr( (G_{11} - K^\top G_{21} - G_{12}K + K^\top G_{22}K) W)
\end{align*}
we set the gradient of the above expression with respect to $K^\top$ to zero using the rule $\nabla_A tr(AB) = B^\top$. This results in the same constant linear feedback policy as before:
\begin{align*}
- 2 W G_{12} + 2 W K_*^\top G_{22} = 0 \\
K_* = G_{22}^{-1} G_{21} \,.
\end{align*}
\fi
