# Supplementary material for: Model-Free Linear Quadratic Control via Reduction to Expert Prediction
Source: arXiv:1804.06021 source file (2018-10-05)
Supplement: Supplementary file 2 [file appendix_state_action_bound.tex]

\begin{lemma}
\label{lem:state-action-bound}
Assume that $T \geq S \ln(3C_1) / \ln (1 + (6C_1)^{-1})$. For any $t=1,2,\dots,T$ with probability at least $1-\delta_2$,
\[
\norm{x_{t}} \le C_X := \frac{\sqrt{2n \log (Tn/\delta_2)}}{1-\sqrt{1-(2C_H)^{-2}}}\,, 
\qquad \norm{a_t} \le C_A := \sqrt{C_H} C_X\;.
%\norm{x_s} \le  \frac{\sqrt{2n C_1 C_H \log (Tn/\delta_2)}}{1-\sqrt{1-(2C_H)^{-2}}} \;.
 \]
\end{lemma}

\subsection{Proof of Lemma~\ref{lem:state-action-bound}}
\label{sec:boundedness_proof}
\begin{proof}
First, we show that states remain bounded. Let $\Gamma_i = A - B K_i$, and let $\Gamma_{(t)}$ be the closed-loop matrix at time step $t$. We have that
\begin{align*}
x_{t+1} &= \Gamma_{(t)} x_t + w_{t} \\
&= \Gamma_{(t)} \Gamma_{(t-1)} x_{t-1} + \Gamma_{(t)} w_{t-1} + w_{t}\\
 &= \dots\\
&= \bigg(\prod_{s=0}^{t} \Gamma_{(t-s)}\bigg) x_0 + \sum_{\tau=0}^{t} \bigg( \prod_{s=0}^{t-\tau-1} \Gamma_{(t-s)} \bigg) w_\tau
\end{align*}
For each policy $K_i$, we have that
$\norm{\Gamma_i^k} \leq C_H^{1/2} \;(1 - (2C_H)^{-1})^{k/2}$. Furthermore, since we run $S$ policies for $T / S$ time steps each, after $t$ time steps there have been at most $\lfloor tS /T \rfloor $ policies. Hence 
\begin{align}
\norm{\prod_{s=1}^{t} \Gamma_{(t+1-s)}} & \leq \bigg( {C_H}^{(S / T)}(1 - (2C_H)^{-1}) \bigg)^{t/2}%\prod_{i=0}^{t^{1/4}-1} (1 + S^{-1})^{i/2} 
\end{align}
By assumption, $T / S \geq \frac{\ln(C_H)}{ \ln (1 + (2C_H)^{-1})}$. Hence ${C_H}^{S/T} \leq 1 + (2C_H)^{-1}$ and 
\[
\norm{\prod_{s=1}^{t} \Gamma_{(t+1-s)}} \leq \big(1 - (2C_H)^{-2}\big)^{t/2} \,.
\]
Given that all noise terms are smaller than $\sqrt{2n \log (Tn/\delta_2)}$ with probability at least $1-\delta_2$, we get for all $s=1,\dots,\tau+1$
\[
\norm{x_{s}} \le \frac{\sqrt{2n \log (Tn/\delta_2)}}{1-\sqrt{1-(2C_H)^{-2}}} \;.
\]
Next, we show that all actions remain bounded. 
% Let $H_*$ be the optimal value matrix, and let $W'$ be a bounded positive semidefinite matrix such that $H_i \prec H_* + W'$.
We have that
\[
K_i^\top K_i \prec (A - BK_i)^\top H_i (A - B K_i) + M + K_i^\top N K_i = H_i \;. % \prec H_* + W' \;.
\]
Thus,
\[
\norm{a_s}^2 \le C_H \norm{x_s}^2 \le  \frac{2n C_H \log (Tn/\delta_2)}{(1-\sqrt{1-(2C_H)^{-2}})^2} \;.
\]
\end{proof}
