# Supplementary material for: Model-Free Linear Quadratic Control via Reduction to Expert Prediction
Source: arXiv:1804.06021 source file (2018-10-05)
Supplement: Supplementary file 3 [file appendix_estimation_old.tex]

 \section{$\beta$-mixing of stable linear dynamical systems}
%%%%%%%%%%%%%%%%%%%%%%%%%%%%%%%%%

\label{sec:app_b}
\newcommand{\an}{b}
\newcommand{\mun}{m}
\newcommand{\Residual}{\mathcal{R}}
\newcommand{\vZ}{\mathbf{Z}}
\newcommand{\Parens}[1]{\left(#1\right)}
\newcommand{\bbE}{\mathbb{E}}
\newcommand{\tv}{\mathrm{tv}}
\newcommand{\Norm}[1]{\left\|#1\right\|}
\newcommand{\vP}{\mathbf{P}}
\newcommand{\pimin}{\pi_*}
\newcommand{\obeta}{\overline{\beta}}

Let $\norm{\cdot}_{\tv}$ denote the total variation norm.
\begin{definition}[$\beta$-mixing]
Let $\{Z_t\}_{t=1,2,\ldots}$ be a stochastic process.
Denote by $Z_{1:t}$ the collection $(Z_1,\ldots,Z_t)$, where we allow $t=\infty$.
Let $\sigma(Z_{i:j})$ denote the sigma-algebra generated by $Z_{i:j}$ ($i\le j$).
The $k^{\rm th}$ $\beta$-mixing coefficient of $\{Z_t\}$, $\beta_k$, is defined by
\begin{align*}
 \beta_k
 & = \sup_{t\ge 1} \EE{ \sup_{B\in\sigma(Z_{t+k:\infty})} |P(B|Z_{1:t})-P(B)| } \\
 & = \sup_{t\ge 1} \EE{ \norm{P_{Z_{t+k:\infty}|Z_{1:t}}(\cdot|Z_{1:t})-P_{Z_{t+k:\infty}}(\cdot)}_{\tv} }\,.
\end{align*}
%A stochastic process
$\{Z_t\}$ is said to be $\beta$-mixing if $\beta_k\ra 0$ as $k\ra\infty$.
In particular, we say that
 a $\beta$-mixing process mixes at an {\em exponential} rate with parameters $\obeta, \alpha , \gamma>0$
 if $\beta_k \le \obeta \exp(-\alpha k^\gamma)$ holds for all $k\ge 0$.
\end{definition}

Note that if $X_t$ is $\beta$-mixing, $Y_t \sim P_{Y|X}(\cdot|X_t)$,
 then the hidden-Markov process $\{(X_t,Y_t)\}$ is also $\beta$-mixing with the same rate
 (see, e.g., the proof of Proposition~4 in \cite{CarChe:Mixing02}
 for an argument that can be used to prove this).

% For a square matrix $A$, we use $\rho(A)$ to denote its spectral radius, and we define its resolvant $R_A(a)$ as $R_A(a) = (a I - A)^{-1}$. 
\begin{lemma}[\cite{tu2017least}] %[Corollary 3.3]
\label{lem:mixing}
Consider a linear dynamical system $x_{t+1}=\Gamma x_t + w_t$, $w_t \sim \cN(0, I_d)$, such that $\rho(\Gamma) < 1$, where $\rho(\cdot)$ is the spectral radius of a matrix.
Fix any $\alpha\in (\rho(\Gamma), 1)$. For any $k\ge 1$ we have
\[
\beta_k \le \frac{\norm{R_{\alpha^{-1} \Gamma}}_{\cH_\infty}}{2} \sqrt{\trace(\Sigma) + \frac{d}{1-\alpha^2}} \alpha^k \;,
\]
where %$\norm{.}_{\cH_\infty}$ denotes the $\cH_\infty$-norm, % (see \citet{tu2017least} for the definition), 
$R_A(a) = (a I - A)^{-1}$, and $\Sigma = \sum_{s=1}^\infty \Gamma^s {\Gamma^s}^\top$ is the steady-state covariance of $x$.
\end{lemma}


\section{Upper bounds for partial sums under $\beta$-mixing}
Let $(X_t)_{t\in [n]}$ be a sequence of random variables. 
For an index set $I\subset [n]$ define $S_I = \sum_{i\in I} X_i$ and $X_I = (X_i)_{i\in I}$. 
Note that $S_I$ is a function of $X_I\in \R^{|I|}$.
By abusing notation we also define
$S_t = S_{[t]}$ for $t\in [n]$.
We are interested in bounding the excursions of $S_n$ over zero, i.e., bounds on $s$ that make the probability of $S_n>s$ small.
Hoeffding's inequality states that 
if $(X_t)_{t\in [n]}$ is a sequence of independent, zero-mean random variables 
taking values in the range $[-\kappa,\kappa]\subset \R$ w.p.1., then
\begin{align}
\label{eq:apx:hoeff}
\Prob{ S_n > s } \le \exp( - s^2 / (2 n \kappa^2) )\,.
\end{align}

We are interested in the case when $(X_t)_t$ is a dependent process, when $X_t\in [-1,1]$ a.s.
To bound the probability of $S_n>s$,
we will use the so-called independent blocks technique \cite{Bernstein27,Yu94}.
%described  by \citet{Yu94} and is attributed to \cite{Bernstein27}.

%========================================================
\newcommand{\bbP}{\mathbb{P}}
\newcommand{\wt}{\widetilde}


We start by defining a partitioning of the set $\{1,2,\ldots,n\}$ determined by the choice of an integral block length $\an$. The partition will have $2 \mun$ blocks, each with integral length $\an$ such that $n - 2 \an < 2 \mun \an \leq n$, and a ``residual block'' at the end: For $j\in [\mun]$, let
%
%
\begin{align*}
	H_j & = \{ i : 2(j-1)\an + 1 \leq i \leq (2j-1)\an\}, \,\quad & \mbox{(``head'')} \\
	T_j & = \{ i: (2j-1)\an + 1 \leq i \leq 2j \an	\}, \, \quad\quad & \mbox{(``tail'')}\\
\end{align*}
while let
\begin{align*}
	\makebox[0pt][l]{$\Residual$}
	\phantom{H_j }
	&
	\makebox[0pt][l]{	
		$= \{ 2\mun \an + 1, \ldots, n\},  $
	}
	\phantom{ 
		= \{ i : 2(j-1)\an + 1 \leq i \leq (2j-1)\an\}, \,\quad
	}
	& \mbox{(``residual'')}
\end{align*}
%
Note that $|\Residual | < 2 \an$.
%
Also, let $H = \cup_{1 \leq j \leq \mun} H_j$ and $T = \cup_{1 \leq j \leq \mun} T_j$.
See Figure~\ref{fig:blocks} for the illustration of this construction.
\begin{figure}
\begin{center}
\begin{tikzpicture}[thick, framed]
%	\draw[|-|] (0,0) -- (14.1,0);
	% Plan:
	% H1
	% T1
	% H2
	% T2
	% dots
	% H_{\mun}
	% T_{\mun}
	% Residual
	
	% H1, T1, H2, T2
	\draw[|-|,thick,red] (0.0,0) coordinate (H11) 	-- coordinate (H1) (1.0,0) coordinate (H12);	
	\draw[|-|,thick,red] (1.1,0) coordinate (T11)  -- coordinate (T1) (2.2,0) coordinate (T12);
	\draw[|-|,thick,red] (2.3,0) coordinate (H21)  -- coordinate (H2) (3.3,0) coordinate (H22);
	\draw[|-|,thick,red] (3.4,0) coordinate (T21)  -- coordinate (T2) (4.4,0) coordinate (T22);
	% dot dot dot
	\fill (5.0,0) circle (1pt);
	\fill (5.1,0) circle (1pt);
	\fill (5.2,0) circle (1pt);
	% Hmun, Tmun, R
	\draw[|-|,thick,red] (5.8,0) coordinate (Hn1) 	-- coordinate (Hn) (6.8,0) coordinate (Hn2);	
	\draw[|-|,thick,red] (6.9,0) coordinate (Tn1)  -- coordinate (Tn) (7.9,0) coordinate (Tn2);
	\draw[|-|,thick,red] (8.0,0) coordinate (R11)  -- coordinate (R1) (8.7,0) coordinate (R12);

	% braces
%	\draw[snake=brace,raise snake=5pt,red]	(H11) -- (H12);
%	\draw[snake=brace,raise snake=5pt,red]	(T11) -- (T12);
	\draw[snake=brace,raise snake=5pt,red]	(H21) -- (H22);
%	\draw[snake=brace,raise snake=5pt,red]	(T21) -- (T22);
%	\draw[snake=brace,raise snake=5pt,red]	(Hn1) -- (Hn2);
%	\draw[snake=brace,raise snake=5pt,red]	(Tn1) -- (Tn2);
%	\draw[snake=brace,raise snake=5pt,red]	(R11) -- (R12);
		
	% labels
	\draw 
	(H1) node[below=2pt] {$H_1$}
	(T1) node[below=2pt] {$T_1$}
	(H2) node[below=2pt] {$H_2$}
	(T2) node[below=2pt] {$T_2$}
	(Hn) node[below=2pt] {$H_{\mun}$}
	(Tn) node[below=2pt] {$T_{\mun}$}
	(R1) node[below=2pt] {${\Residual}$}
	(H2) node[above=8pt] {$\an$}
	;
%	\draw[|-|,label=above:$s\le3$] (0,0) -- (14.1,0) {2};
\end{tikzpicture}
\end{center}
\caption[Construction of Independent Blocks]{The structure of the block construction.}
\label{fig:blocks}
\end{figure}


%========================================================

We have $S_n =S_H+S_T + S_{\Residual}$.
Thus, to bound the probability that $S_n>s$
 it is enough to bound the probabilities that $S_H>s/2$ and $S_T>s/2$, and combine these with
 $S_{\Residual} \le 2b$, which holds with probability one. We first bound the probability that $S_H$ is large.
The bound for $S_T$ works in an entirely analogous fashion.
To bound this probability, we appeal to a consequence of Corollary~2.7 form \cite{Yu94}.
%\citep[a consequence of][Corollary 2.7]{Yu94}.

Let $\bbP$ denote the joint distribution of $(X_{H_j} : j \in [\mun])$; 
let $\bbP_s$ be its marginal over $X_{H_j}$, and let
$\bbP_{1:j+1}$ be its marginal over
$(X_{H_1},X_{H_2},\dotsc,X_{H_{j+1}})$.
Let $\wt\bbP$ be the product distribution formed from the marginals
$\bbP_1,\bbP_2,\dotsc,\bbP_{\mun}$.
Corollary~2.7 of \cite{Yu94} implies that for any Borel-measurable set $E\subset \R^{H}$,
\[
  |\bbP(E) - \wt\bbP(E)| \leq (\mun-1) \beta_m(\bbP)
\]
where
\[
  \beta_m(\bbP)
  :=
  \max_{1 \leq j \leq \mun-1}
  \EE{{
    \Norm{
      \bbP_{1:j+1}(\cdot\,|X_{H_1},X_{H_2},\dotsc,X_{H_j}) - \bbP_{j+1}
    }_{\tv}
  }}
  \,.
\]
Clearly, if $\beta_d$ is the $d$th $\beta$-mixing coefficient of $(X_t)_t$, 
$\beta_m(\bbP)\le \beta_b$ (the size of the ``gap'' between successive blocks is $b$).

Now take $E= \{ x\in \R^H \,:\, \sum_{t\in H} x_t > s/2 \}$ and
let $(\wt S_{H_j})_{j\in [\mun]}$ be a sequence of independent random variables
such that $\wt S_{H_j}\sim \bbP_j$.
Then, $\wt S_{H_j} \in [-b,b]$ a.s.,
$\wt\bbP(E) = \Prob{ \sum_{j\in [\mun]} \wt S_{H_j} > s/2 } \le \exp( - s^2 / (8 \mun b^2) )
\le \exp( - s^2 / (4 b n) )$, where the last inequality used that $2mb\le n$.
Equating the right-hand side with $\delta$ and inverting for $s$, we get that
\begin{align*}
s =  2\sqrt{ b n \log(1/\delta)}\,,
\end{align*}
Putting things together, we get that 
\begin{align*}
\Prob{ S_H > \sqrt{bn \log(1/\delta)} } \le \delta + (m-1)\beta(\bbP)\le \delta + n\beta_b \,.
\end{align*}
Similarly,
\begin{align*}
\Prob{ S_T > \sqrt{bn \log(1/\delta)} } \le \delta + (m-1)\beta(\bbP)\le \delta + n\beta_b 
\end{align*}
and thus outside of an event of probability at most $2\delta + 2n\beta_b$,
\begin{align*}
S = S_H+S_T + S_{\Residual} \le 2\sqrt{bn \log(1/\delta)} + 2b\,.
\end{align*}
Now, assume that $\beta_b \le \obeta \exp(-\alpha b)$ holds for some $\obeta, \alpha>0$ parameters.
Setting $\delta = n \obeta \exp(-\alpha b)$ and solving for $b$ we get \todoc{We need to round this; edge cases, ..}
\begin{align*}
b =  \frac{1}{\alpha}\log\left( \frac{2\obeta n }{\delta} \right)\,.
\end{align*}
Plugging this into the previous display gives that with probability at most $4\delta$,
\begin{align*}
S
& \le  2\sqrt{\frac{n}{\alpha}\log\left( \frac{2\obeta n }{\delta} \right)\, \log\left(\frac1\delta\right)} 
+ \frac{2}{\alpha}\log\left( \frac{2\obeta n }{\delta} \right)
 \le 2  \log\left( \frac{2\obeta n }{\delta} \right) \left\{ \sqrt{\frac{n}{\alpha}} 
+ \frac{1}{\alpha}\right\}\,.
\end{align*}
where the last inequality uses that $2\obeta n \ge 1$, which we may assume without loss of generality. \todoc{The last overestimate is used to simplify the final result.}

\if0

==========================================

\todoc[inline]{Sketch for now.. but it has the essential things.. }


Bin Yu's result gives
\begin{align*}
\left|\Prob{ \sum_{i=1}^m S_{H_i}>x} - \Prob{ \sum_{i=1}^m S_{H_i}' > x } \right|\le \beta_b \frac{n}{2}\,,
\end{align*}
where $n/2 = m \times b$.
This implies that 
\begin{align*}
\Prob{ \sum_{i=1}^m S_{H_i}>x}
&  \le \Prob{ \sum_{i=1}^m S_{H_i}' > x } + \beta_b \frac{n}{2} 
  \le e^{-2mx^2/(m b^2)} + c e^{-\alpha b} \frac{n}{2} \,.
\end{align*}
Choose $x$ so that $\delta/2 = e^{-2 x^2/(mb^2)}$. Solving for $x$, we get
\begin{align*}
x 
 = b \sqrt{m\log(2/\delta)/2} 
 = \sqrt{m b^2 \log(2/\delta)/2} 
 = \frac12 \sqrt{n b \log(2/\delta)}\,.
\end{align*}
Now set $b$ so that $c e^{-\alpha b} \frac{n}{2}=\delta/2$. Solving for $b$, we get
\begin{align*}
b = \frac{1}{\alpha}\log\left( \frac{2cn}{\delta} \right)\,.
\end{align*}
Repeating this calculation for $\sum_{i=1}^m S_{T_i}$ and combining the inequalities obtained
gives the following result:
With probability $1-\delta$,
\begin{align*}
\frac1n S_n
 = \frac1n \left(\sum_{i=1}^m S_{H_i}+\sum_{i=1}^m S_{T_i} \right)
\le  \sqrt{ \frac{b \log(4/\delta)}{n} } 
\le  \sqrt{ \frac{\log( (2cn)/\delta) \log(4/\delta)}{\alpha n} }\,.
\end{align*}
 
\fi

%%%%%%%%%%%%%%%%%%%%%%%%%%%%%


\section{Estimating H}


\subsection{Bounding the smallest eigenvalue of $\E[\phi_t(\phi_t - \phi_{t+1}^\top) + (\phi_t - \phi_{t+1})\phi_t^\top]$}
\label{sec:app_b1}

To bound the smallest eigenvalue of $\E[\phi_t(\phi_t - \phi_{t+1}^\top) + (\phi_t - \phi_{t+1})\phi_t^\top]$, we adapt the results of \cite{tu2017least} who analyze $\E(\phi \phi^\top)$ in the context of LSTD for discounted LQ control.
%We first state a number of useful results from \cite{tu2017least}. Let $(x_k )_{k=1}^{\infty}$ be a discrete-time vector-valued process adapted to a filtration $(\cF_t)_t$.  %$x_1^t := (x_k)_{k=1}^t$ be a sequence of states. 
%For an integer $k$, define the $\beta$-mixing coefficient $\beta(k)$ with respect to the steady-state distribution $\mu$ as
%\[
%\beta(k) := \sup_{t\ge 1} \E[ \norm{\P_{x_{t+k}}(\cdot|\cF_t) -\mu }_{\text{tv}}] \;,
%\] 
%where $\norm{.}_{\text{tv}}$ denotes the total-variation norm,
%and $\P_{x_{t+k}}(\cdot|\cF_t)$ is the conditional distribution of $x_{t+k}$ given $\cF_t$. We next state mixing time results for a stable linear dynamical system. 

For any positive $\omega$ define the small-ball probability $P(\omega)$ as 
\[
P(\omega) := \inf_{\norm{v}=1} \P_{\mu} (\abs{\ip{v}{x}} \ge \omega ) \;.
\]
We use the following theorem of \cite{tu2017least}, which is a generalization of the result of \cite{Koltchinskii-Mendelson-2013}. 
\begin{theorem}
\label{thm:lambdalower}
Fix $\delta\in (0,1)$. Suppose that $(x_k)_{k=1}^\infty$ is a discrete-time stochastic process with stationary distribution $\mu$ that satisfies $\beta_k\le D \alpha^k$ for some $D>0$ and $\alpha\in (0,1)$. Suppose that there exists a $\omega$ satisfying $P(\omega) > 0$. Furthermore, suppose that $\tau$ satisfies
\[
\tau \ge \frac{\log(2 D \tau/\delta)}{1-\alpha} \left( \max\left\{\frac{1024 \E_{\mu} \norm{x}^2}{\omega^2 P^2(\omega)} , \frac{32}{P^2(\omega)} \log\left( \frac{4}{\delta(1-\alpha)} \log \left( \frac{2D\tau}{\delta} \right) \right) \right\} +1 \right) \;.
\]
Then, with probability at least $1-\delta$,
\[
\lambda_{\text{min}} \left( \frac{1}{\tau} \sum_{k=1}^\tau x_k x_k^\top \right) \ge \frac{\omega^2 P(\omega)}{8} \;.
\]
\end{theorem}

We are now ready to state and prove Lemma~\ref{lem:lambdaLower}. 
\begin{proof}
We apply Theorem~\ref{thm:lambdalower} to the process $\phi(x_t) - \phi(x_{t+1})$. In Section~\ref{sec:small_ball}, we show that the small-ball probability of this process is bounded as
\beq
\label{eq:vphi}
\Prob{\abs{\ip{v}{\phi(x_{t+1}) - \phi(x_t)}} \ge 1 } \ge 1/324 \;,
\eeq
where $\norm{v} = 1$. 
Next, we upper-bound the second moment,
\begin{align}
\label{eq:up2moment}
\notag
\EE{\norm{\phi(x_{t+1}) - \phi(x_t)}^2} &\le 4\EE{\norm{\phi(x_t)}^2}\\ 
\notag
&= 4\EE{\norm{x_t}^4}\\ 
\notag
&= 8 \norm{\Sigma^{1/2}}_F^2 + 4\trace(\Sigma^{1/2})^2\\ 
&\le 12 \trace(\Sigma^{1/2})^2 \;.
\end{align}
Given \eqref{eq:vphi} and \eqref{eq:up2moment}, we get the desired lower bound from Theorem~\ref{thm:lambdalower}. 
\end{proof}

\subsection{Bounding the small-ball probability}
\label{sec:small_ball}

In this section we bound the small-ball probability $P(\omega) = \inf_{\norm{v}=1} \P_{\mu} (\abs{\ip{v}{\phi' - \phi}} \ge \omega )$ for $\omega = 1$.  We assume identity noise covariance $W=I$ for simplicity; with known $W \succ 0$, we can always change coordinates to whiten the noise. 
We first state a useful result for fourth moment of multivariate Gaussians. A proof can be found in \citep{tu2017least}. 
\begin{proposition}
\label{prop:moment4}
Let $g\sim \cN(0,I)$, and let $F,F'$ be two fixed symmetric matrices. We have that
\[
\EE{g^\top F g g^\top F' v} = 2\ip{F}{F'} + \trace(F)\trace(F') \;.
\]
\end{proposition}

Write $x = \Sigma^{1/2} g$ and $x' = \Gamma \Sigma^{1/2} g + g'$, where $g\sim \cN(0,I)$ and $g'\sim \cN(0,I)$ are independent. For any unit norm vector $v$ of appropriate dimension, let $V = \mat(v)$, where $\mat$ is the inverse of the $\vect$  operation. Define
\begin{align*}
f_v(g,g') &= \ip{v}{\phi' - \phi} = \ip{v}{\phi(\Gamma \Sigma^{1/2} g + g') - \phi(\Sigma^{1/2} g)} \\
&= (g'^\top + g^\top \Sigma^{1/2} \Gamma^\top) V (\Gamma \Sigma^{1/2} g + g') - g^\top \Sigma^{1/2} V \Sigma^{1/2} g \;.
\end{align*}
Function $f_v$ is a degree two polynomial in $g$ and $g'$. Next we show the following lower bound for the second moment of $f_v$,
\[
\E(f_v(g,g')^2) \ge 2 \;.
\]
We decompose the expectation as $\E(f_v(g, g')^2) = T_1 + T_2 + T_3$, where
% \begin{align*}
% \E(f_v(g,g')^2) &= \EE{((g'^\top + g^\top \Sigma^{1/2} \Gamma^\top) V (\Gamma \Sigma^{1/2} g + g'))^2} + \EE{(g^\top \Sigma^{1/2} V \Sigma^{1/2} g)^2}\\ 
% &\qquad-2 \EE{(g^\top \Sigma^{1/2} V \Sigma^{1/2} g)((g'^\top + g^\top \Sigma^{1/2} \Gamma^\top) V (\Gamma \Sigma^{1/2} g + g'))} \;.
% \end{align*}
% Let
\begin{align*}
T_1 &= \EE{((g'^\top + g^\top \Sigma^{1/2} \Gamma^\top) V (\Gamma \Sigma^{1/2} g + g'))^2} \\
 T_2 &= \EE{(g^\top \Sigma^{1/2} V \Sigma^{1/2} g)^2}\\
 T_3 &= -2 \EE{(g^\top \Sigma^{1/2} V \Sigma^{1/2} g)((g'^\top + g^\top \Sigma^{1/2} \Gamma^\top) V (\Gamma \Sigma^{1/2} g + g'))} \;.
\end{align*}
For the first term, we have
\begin{align}
\label{eq:T1}
\notag
T_1 &= \EE{(g'^\top V g' + g^\top \Sigma^{1/2} \Gamma^\top V \Gamma \Sigma^{1/2} g + 2 g'^\top V \Gamma \Sigma^{1/2} g)^2} \\
\notag
&= \EE{(g'^\top V g')^2} + \EE{(g^\top \Sigma^{1/2} \Gamma^\top V \Gamma \Sigma^{1/2} g)^2} + 4 \EE{(g'^\top V \Gamma \Sigma^{1/2} g)^2}\\
\notag
&\qquad\qquad+ 2\EE{(g'^\top V g')(g^\top \Sigma^{1/2} \Gamma^\top V \Gamma \Sigma^{1/2} g)} + 4\EE{(g'^\top V g')(g'^\top V \Gamma \Sigma^{1/2} g)}\\ 
\notag
&\qquad\qquad + 4\EE{(g^\top \Sigma^{1/2} \Gamma^\top V \Gamma \Sigma^{1/2} g)(g'^\top V \Gamma \Sigma^{1/2} g)}\\
\notag
&= 2\norm{V}_F^2 + \trace(V)^2 + 2\norm{\Sigma^{1/2}\Gamma^\top V \Gamma \Sigma^{1/2}}_F^2 + \trace(\Sigma^{1/2}\Gamma^\top V \Gamma \Sigma^{1/2})^2 &\text{Proposition~\eqref{prop:moment4} and  $g\perp g'$}\\ 
\notag
&\qquad\qquad+ 4 \EE{(g'^\top V \Gamma \Sigma^{1/2} g)^2} + 2\EE{g'^\top V g'}\EE{g^\top \Sigma^{1/2} \Gamma^\top V \Gamma \Sigma^{1/2} g}\\
&= 2\norm{V}_F^2 + \trace(V)^2 + 2\norm{\Sigma^{1/2}\Gamma^\top V \Gamma \Sigma^{1/2}}_F^2 + \trace(\Sigma^{1/2}\Gamma^\top V \Gamma \Sigma^{1/2})^2\\ 
\notag
&\qquad\qquad+ 4 \norm{\Sigma^{1/2}\Gamma^\top V}_F^2 + 2\trace(V)\trace(\Sigma^{1/2}\Gamma^\top V \Gamma \Sigma^{1/2})\,,
\end{align}
where in the last step we used
\[
\EE{(g'^\top V \Gamma \Sigma^{1/2} g)^2} = \EE{g'^\top V \Gamma \Sigma^{1/2} g g^\top \Sigma^{1/2} \Gamma^\top V g'} = \trace(\Sigma^{1/2} \Gamma^\top V^2 \Gamma \Sigma^{1/2}) = \norm{\Sigma^{1/2} \Gamma^\top V}_F^2 \;.
\]
For the second term, we have
\beq
\label{eq:T2}
T_2 = 2\norm{\Sigma^{1/2} V \Sigma^{1/2}}_F^2 + \trace(\Sigma^{1/2} V \Sigma^{1/2})^2 \;.
\eeq
For the third term, we have
\begin{align}
\label{eq:T3}
\notag
T_3 &= -2 \EE{(g^\top \Sigma^{1/2} V \Sigma^{1/2} g)(g'^\top V g')} -2 \EE{(g^\top \Sigma^{1/2} V \Sigma^{1/2} g) (g^\top \Sigma^{1/2} \Gamma^\top V \Gamma \Sigma^{1/2} g)}\\ 
\notag
&\qquad\qquad-4 \EE{(g^\top \Sigma^{1/2} V \Sigma^{1/2} g) (g'^\top V \Gamma \Sigma^{1/2} g)} \\
&= -2 \trace(\Sigma^{1/2} V \Sigma^{1/2}) \trace(V) -4 \ip{\Sigma^{1/2}V\Sigma^{1/2}}{\Sigma^{1/2}\Gamma^\top V \Gamma \Sigma^{1/2}} -2\trace(\Sigma^{1/2}V\Sigma^{1/2})\trace(\Sigma^{1/2}\Gamma^\top V \Gamma \Sigma^{1/2}) \;.
\end{align}
By \eqref{eq:T1}, \eqref{eq:T2}, and \eqref{eq:T3}, we get that
\begin{align*}
\E(f_v(g,g')^2) &= (\trace(\Sigma^{1/2}\Gamma^\top V \Gamma \Sigma^{1/2}) - \trace(\Sigma^{1/2} V \Sigma^{1/2}) + \trace(V) )^2 + 2\norm{\Sigma^{1/2}\Gamma^\top V \Gamma \Sigma^{1/2} - \Sigma^{1/2} V \Sigma^{1/2}}_F^2\\ 
&\qquad\qquad+ 2\norm{V}_F^2 + 4\norm{\Sigma^{1/2} \Gamma^\top V}_F^2 \\
&\ge 2 \norm{V}_F^2 = 2\;.
\end{align*}
Using the above lower bound and Lemma~4.6 of \cite{tu2017least},
\beq
\Prob{\abs{\ip{v}{\phi(x_{t+1}) - \phi(x_t)}} \ge 1 } \ge 1/324 \;.
\eeq
